# Supplementary material for: The Diversity of Type Ia Supernovae from Broken Symmetries
Source: arXiv:0907.0708 source file (2009-07-03)
Supplement: Supplementary file 1 [file kasen_supplement.pdf]

# Supplementary Material

## 1. Explosion Simulations

For simulating the explosion process, we employed a code[12,31,32] that treated the hydrodynamics in a higher-order Godunov scheme[33] and followed the propagation of the thermonuclear flames in a level-set approach[34]. The effects of unresolved turbulence driving the propagation of the deflagration flame were accounted for by a subgrid-scale turbulence model[35]. This approach allowed for a self-consistent treatment of the flame propagation while avoiding tunable parameters.

The deflagration level set was initiated representing a collection of spherical ignition sparks of radius 6 km distributed around the WD center, within a certain solid angle. From 20 to 150 ignition points were considered, randomly distributed from the center out to ~300 km and in a solid angle whose opening varied from $60^o$ to $360^o$.

(see Table 1 for the ignition configurations of each model). Consequently, the ignition region forms a cone with the apex at the center of the WD. Inside this region, the sparks were randomly placed in angular direction. Their distribution in radial direction was randomly drawn from a Gaussian distribution. The apex angles of the cones and the standard deviations of the Gaussian distributions are listed in Table 1.

From these ignition configurations, the deflagration flame fronts evolved subject to buoyancy instabilities on large scales and driven by turbulent motions generated on smaller scales. The deflagration flames propagated from the center of the WD outwards

and released energy, expanding the star. Until getting close to the surface of the WD, the deflagration flame is deformed on large scales by turbulence and thus its propagation is accelerated, but its microscopic structure remains "laminar", with its width and speed determined by radiative diffusion and conduction. Therefore it is stable against detonation. However, as the star expands and the flame burns towards its edge, the density directly ahead of the flame declines. The laminar flame structure becomes thicker and eventually small eddies can penetrate into the burning region and mix hot ash with cold fuel without immediately burning. This mixing process first begins when the Karlovitz number, Ka becomes greater than unity[36], and it has long been speculated that a transition to detonation, were it to happen, would happen here[37]. However, more recent studies[21,22] suggest that the first structures to form at the transition to distributed burning are too small to detonate. Greater mixing, and therefore a lower density and higher Karlovitz number are required. The largest mixed structures are formed when the eddy turnover time on the integral scale for the turbulence is equal to the nuclear burning time for the mixture, i.e., Damköhler number ~ 1. The effects of intermittency will raise this value some[38] to perhaps Da ~ 10. Estimating the nuclear time scale with a small reaction network and assuming turbulent energies appropriate to the supernova[39], this corresponds to Ka ~ 500.

This possibility of a deflagration-to-detonation transition (DDT) was implemented in the models by determining Ka in each zone near the flame surface based upon the turbulent energy as derived from the subgrid-scale turbulence model. Here Ka is defined as Ka = $(\delta/L_{Gib})^{1/2}$ where $\delta$ is the laminar flame width, and the Gibson length, $L_{Gib}$ =

$[S_{lam}/u'(\Delta x)]^3\Delta x$, with $S_{lam}$, the laminar flame speed and u', the turbulent *rms* fluctuation speed on the scale of the computational grid Δx. For a DDT to occur in our simulation, we required a minimal Karlovitz number and a certain range of fuel densities ahead of the flame, as given in Table 2. We considered five different values of critical Karlovitz number. Most models used a value in the most physically plausible range (Ka = 250, 750) while other models explored more extreme values (Ka = 1, 1500, 2250).

Once the flame fronts reached the critical conditions for detonation, a level set representing a detonation was initiated at the corresponding location. If other features of the flame reached critical DDT conditions, further detonations were initialized there on the basis of the same level set. Thus, a sequence of DDTs was possible and indeed realized in all models. The detonation level set was then propagated with an appropriate detonation velocity[40], exhausting most of the remaining fuel. The level-set treatment of the detonation allowed us to prevent it from unphysically crossing ash regions left behind by the preceding deflagration phase.

Each thermonuclear supernova explosion model is now specified by one of the deflagration ignitions configurations listed in Table 1 and one of the DDT conditions of Table 2. In total, 44 models were computed.

Depending on the fuel density ahead of the flame, the C+O material of the WD was converted to a nuclear statistical equilibrium composition (NSE; modeled as a temperature-and density-dependent mixture of $^{56}$Ni and alpha-particles), or to

intermediate mass elements (modeled by a representative nucleus of A=30 and a nuclear binding energy of 8.17906 x $10^{18}$ erg $g^{-1}$), or to oxygen. Electron captures in the NSE were accounted for in a parameterized way allowing us to differentiate radioactive $^{56}$Ni from stable iron group elements.

For select models, we carried out detailed post-processing nucleosynthesis calculations using Lagrangian tracer particles and a full nuclear network (see Figure 1 for two models discussed in the main text). For one of the more representative models (D2D_iso_06_dc1) we tabulated the detailed compositions comprising each of the coarse groups followed in the explosion calculations. These tables were used for the remaining models to interpolate the abundances of all elements, a prerequisite for the spectrum synthesis modeling described below. The light curves are less sensitive to the details of the abundance interpolation.

The explosion simulations were run in cylindrical (r-z) geometry and a spatial resolution of 512x1024. Imposing rotational symmetry along the z-axis, the full star was represented in this two-dimensional setup. The hydrodynamical evolution of each model was followed for 100 seconds, well after burning had ceased and at which point the gravitational and internal energy densities were small (< 1%) relative to the kinetic energy density. At this time, the velocity structure was homologous (velocity proportional to radius) to better than a percent, indicating that the remnant had reached the phase of free-expansion.

The explosion models all assumed the progenitor star had solar metallicity. To explore how varations in metallicity may influence the light curve, we changed the composition of the debris structure in each explosion model to reflect certain nucleosynthetic results. Timmes[29] showed in an analytical calculation that a higher metallicity leads to a greater production of stable iron group elements ($^{54}Fe$ and $^{58}Ni$) at the expense of $^{56}Ni$. We therefore varied the $^{56}Ni$ mass according to $M_{ni}(Z) = M_{ni}(Z=1) * (1 - 0.057\ (Z-1))$ , where the metallicity was changed to Z = 3 and Z = 0.3 times solar. The trace abundance of metals in unburned or partially burned material, which has some influence on the ejecta opacity, was also changed to reflect the progenitor metalicity. This approach does not account for the effect metallicity may have on the structure of the white dwarf, or on the dynamics of the explosion.

**2. Radiative Transfer Calculations**

Light curves and spectra of the models were computed using the multi-wavelength time-dependent radiative transfer code SEDONA[19], which uses a Monte Carlo approach to solve the transport equation in arbitrary geometries. The final structure of each explosion model described above was remapped to a lower resolution (64x128) regular cylindrical grid to provide the initial conditions for the transfer code. SEDONA assumes the subsequent dynamics are given by homologous expansion and self-consistently calculates the temperature structure evolution by balancing sources of radiative heating and cooling.

The light curves of SNe Ia are powered by the radioactive chain $^{56}Ni \rightarrow {}^{56}Co \rightarrow {}^{56}Fe$. The decay releases primarily ~1 MeV gamma-rays, which deposit their energy in the

ejecta mainly through Compton scattering and photo-electric absorption. The SEDONA code includes a detailed multi-wavelength transport scheme treating the emission, propagation, and absorption of gamma-rays. This provided the instantaneous rate and geometry of radioactive energy deposition, as well as predictions for the emergent gamma-ray light curves and spectra.

Absorbed radioactive energy was assumed to be locally and instantaneously reprocessed into optical/UV photons, whose propagation was followed using a Monte Carlo method. Detailed non-grey opacities were applied, including the aggregate effects of over 10 million bound-bound line transitions[41] treated in the expansion opacity formalism[42]. Atomic level populations were calculated assuming local thermodynamic equilibrium (LTE), typically a reasonable approximation for SNe Ia in the earlier epochs[43]. The radiation field, on the other hand, was not required to be in LTE, and an equivalent two-level equivalent atom (ETLA) formalism was used for the line source function: $S = (1 - \varepsilon) J + \varepsilon B$, where $\varepsilon$ is the ratio of absorptive opacity to total (scattering plus absorptive) opacity. A constant value $\varepsilon = 0.3$ was used for all lines to approximate non-LTE effects based on comparison to previous line branching calculations.

The most significant uncertainties in the light curve calculations relate to uncertainties in the calculation of the complex opacities/emissivities, in particular the likely inaccuracy and/or incompleteness of the atomic line database, and the limitations of the expansion opacity and ETLA formalisms. In the future, self-consistent multi-dimensional non-LTE calculations will help refine the quantitative accuracy of the models.

.

**References**

[31] Röpke, F. K., Following multi-dimensional type Ia supernova explosion models to homologous expansion. Astron. Astrophys. 432, 969–983 (2005).

[32] Röpke, F. K., and Niemeyer, J. C. Delayed detonations in full-star models of type Ia supernova explosions. Astron. Astrophys. 464, 683–686 (2005).

[33] Fryxell, B. A., and Müller, E. Hydrodynamics and nuclear burning. MPA Green Report 449 (1989).

[34] Reinecke, M., Hillebrandt, W., Niemeyer, J. C., Klein, R., and Gröbl, A. A new model for deflagration fronts in reactive fluids. Astron. Astrophys. 347, 724–733 (1999).

[35] Niemeyer, J. C., and Hillebrandt, W. Turbulent Nuclear Flames in Type Ia Supernovae. Astrophys. J. 452 769–778 (1995).

[36] Peters, N. in Turbulent Combustion, Cambridge Univ. Press, p. 78 (2000).

[37] Niemeyer, J. C., and Woosley, S. E., The Thermonuclear Explosion of Chandrasekhar Mass White Dwarfs, Astrophys. J., 475, 740–753, (1997).

[38] Pan, L., Wheeler, J. C., and Scalo, J., The Effects of Turbulent Intermittency on the deflagration to Detonation Transition in Type Ia Supernova Explosions, Astrophys. J., 681, 470–481 (2008).

[39] Röpke, F. Flame Driven Deflagration to Detonation Transitions in Type Ia Supernovae, Astrophys. J., 668, 1103–1108 (2007).

[40] Golombek, I., and Niemeyer, J. C. A model for multidimensional delayed detonations in SN Ia explosions. Astron. Astrophys. 438, 611–616 (2005).

[41] Kurucz, R. Atomic Data for Opacity Calculations, CD-ROM 1, Cambridge: Smithsonian Astrophysical Observatory (1993).

[42] Eastman, R., and Pinto, P. Spectrum Formation in Supernovae: Numerical Techniques. Astrophys. J., 412, 731-751 (1993).

[43] Baron E., Hauschildt, P., Nugent, P., and Branch, D. Non-local Thermodynamic Equilibrium Effects in Modeling of Supernovae near Maximum Light. Mon. Not. R. Astron. Soc., 283, 297-315 (1996).

**Table 1: Deflagration ignition configurations.** The half apex angle of the cone centered on the WD in which the ignition is assumed to take place is denoted by α.

| Ignition setup | Number of ignition kernels | Minimal distance of kernels [kernel radii] | cos(α) | Standard deviation [km] |
|---|---|---|---|---|
| DD2D_iso_01 | 20 | 1.0 | -1.0 | 150.0 |
| DD20_iso_02 | 50 | 0.8 | -1.0 | 150.0 |
| DD2D_iso_03 | 60 | 0.7 | -1.0 | 150.0 |
| DD2D_iso_04 | 80 | 0.8 | -1.0 | 150.0 |
| DD2D_iso_05 | 90 | 0.7 | -1.0 | 150.0 |
| DD2D_iso_06 | 100 | 0.1 | -1.0 | 150.0 |
| DD2D_iso_07 | 100 | 0.5 | -1.0 | 150.0 |
| DD2D_iso_08 | 150 | 0.3 | -1.0 | 150.0 |
| DD2D_asym_01 | 120 | 0.3 | -1.0 | 75.0 |
| DD2D_asym_02 | 105 | 0.3 | -0.75 | 75.0 |
| DD2D_asym_03 | 90 | 0.3 | -0.50 | 75.0 |
| DD2D_asym_04 | 75 | 0.3 | -0.25 | 75.0 |
| DD2D_asym_05 | 60 | 0.3 | 0.0 | 75.0 |
| DD2D_asym_06 | 45 | 0.3 | 0.25 | 75.0 |
| DD2D_asym_07 | 30 | 0.3 | 0.50 | 75.0 |
| DD2D_asym_08 | 15 | 0.3 | 0.75 | 75.0 |

**Table 2: Criteria for deflagration-to-detonation transitions**

| DDT criterion (dc) | $Ka_{min}$ | $\rho_{min}$ [$10^7$ g $cm^{-3}$] | $\rho_{max}$ [$10^7$ g $cm^{-3}$] |
|---|---|---|---|
| 1 | 1.0 | 0.6 | 1.75 |
| 2 | 250.0 | 0.6 | 1.20 |
| 3 | 750.0 | 0.6 | 1.20 |
| 4 | 1500.0 | 0.6 | 1.20 |
| 5 | 2250.0 | 0.6 | 1.20 |
